# Supplementary material for: Spectrally reconfigurable quantum emitters enabled by optimized fast modulation
Source: arXiv:2003.12591 ancillary file (2020-07-28)
Supplement: Supplementary file 1 [file Supplementary_Information.pdf]

# Supplementary Information for “Spectrally reconfigurable quantum emitters enabled by optimized fast modulation”

Daniil M. Lukin,<sup>†1</sup> Alexander D. White,<sup>†1</sup> Rahul Trivedi,<sup>1</sup> Melissa A. Guidry,<sup>1</sup> Naoya Morioka,<sup>2</sup> Charles Babin,<sup>2</sup> Öney O. Soykal,<sup>3</sup> Jawad Ul-Hassan,<sup>4</sup> Nguyen Tien Son,<sup>4</sup> Takeshi Ohshima,<sup>5</sup> Praful K. Vasireddy,<sup>6</sup> Mamdouh H. Nasr,<sup>6</sup> Shuo Sun,<sup>1</sup> Jean-Philippe W. MacLean,<sup>1</sup> Constantin Dory,<sup>1</sup> Emilio A. Nanni,<sup>6</sup> Jörg Wrachtrup,<sup>2</sup> Florian Kaiser,<sup>2</sup> and Jelena Vučković<sup>1</sup>

<sup>†</sup>*These authors contributed equally*

<sup>1</sup>*E. L. Ginzton Laboratory, Stanford University, Stanford, California 94305, USA*

<sup>2</sup>*3rd Institute of Physics, University of Stuttgart and Institute for Quantum Science and Technology IQST, 70569, Stuttgart, Germany*

<sup>3</sup>*Booz Allen Hamilton, McLean, VA, 22102 USA*

<sup>4</sup>*Department of Physics, Chemistry and Biology, Linköping University, SE-58183, Linköping, Sweden*

<sup>5</sup>*National Institutes for Quantum and Radiological Science and Technology, Takasaki, Gunma 370-1292, Japan*

<sup>6</sup>*SLAC National Accelerator Laboratory, Stanford University, 2575 Sand Hill Road, Menlo Park, California 94025, USA*

## Contents

|          |                                                                                                         |           |
|----------|---------------------------------------------------------------------------------------------------------|-----------|
| <b>1</b> | <b>Details of the experimental setup</b>                                                                | <b>5</b>  |
| <b>2</b> | <b>Additional measurements with DC and AC Stark tuning</b>                                              | <b>6</b>  |
| 2.1      | Spectral stability and Stark tuning of the negatively charged $k$ - and $h$ - $V_{\text{Si}}$ in 4H-SiC | 6         |
| 2.2      | Investigating nonlinearity of Stark shift near 0 V bias . . . . .                                       | 7         |
| 2.3      | Observation of Floquet states in $h$ - $V_{\text{Si}}$ . . . . .                                        | 7         |
| 2.4      | Large amplitude drive . . . . .                                                                         | 10        |
| 2.5      | Direct comparison of spectral stability for modulated and unmodulated $V_{\text{Si}}$ . . . .           | 10        |
| <b>3</b> | <b>Scattering matrices for the modulated two-level system</b>                                           | <b>12</b> |
| 3.1      | Single-photon scattering . . . . .                                                                      | 13        |
| 3.2      | Two-photon scattering: . . . . .                                                                        | 15        |
| <b>4</b> | <b>Floquet engineering</b>                                                                              | <b>16</b> |
| 4.1      | Floquet eigenstates . . . . .                                                                           | 16        |
| 4.2      | Floquet state engineering . . . . .                                                                     | 18        |
| 4.3      | Realizable spectra . . . . .                                                                            | 19        |
| 4.4      | Experimental details of photon color-superpositions . . . . .                                           | 20        |
| <b>5</b> | <b>Signature of ground state interference in <math>g^{(2)}(\tau)</math></b>                             | <b>20</b> |

|          |                                                                                |           |
|----------|--------------------------------------------------------------------------------|-----------|
| 5.1      | Theoretical model for the $h$ - $V_{\text{Si}}$ structure . . . . .            | 20        |
| 5.2      | Observation of interference of multiple ground states via $g^{(2)}$ . . . . .  | 24        |
| <b>6</b> | <b>Ramsey interference experiment</b>                                          | <b>25</b> |
| 6.1      | Experimental details . . . . .                                                 | 25        |
| 6.2      | Ramsey interference contrast in a modulated TLS . . . . .                      | 26        |
| <b>7</b> | <b>Spontaneous decay of a spectrally-optimized photon</b>                      | <b>27</b> |
| <b>8</b> | <b>Proposed applications for rapidly modulated quantum emitters</b>            | <b>27</b> |
| 8.1      | Aperiodic modulation for bandwidth expansion . . . . .                         | 28        |
| 8.2      | Inhomogeneous broadening compensation in strongly coupled cavity QED . . . . . | 31        |
| <b>9</b> | <b>References</b>                                                              | <b>33</b> |

## List of Supplementary Figures

|   |                                                                                    |    |
|---|------------------------------------------------------------------------------------|----|
| 1 | Optical experimental setup . . . . .                                               | 5  |
| 2 | Electrical experimental setup . . . . .                                            | 6  |
| 3 | DC Stark tuning characteristics of the $h$ - $V_{\text{Si}}$ . . . . .             | 8  |
| 4 | DC Stark tuning characteristics of the $k$ - $V_{\text{Si}}$ . . . . .             | 9  |
| 5 | Confirming the non-hysteretic nature of the DC Stark shift near 0 V bias . . . . . | 9  |
| 6 | Floquet eigenstates of the $h$ - $V_{\text{Si}}$ under sinusoidal drive . . . . .  | 10 |
| 7 | Large amplitude drive of $k$ - $V_{\text{Si}}$ . . . . .                           | 11 |

|    |                                                                                              |    |
|----|----------------------------------------------------------------------------------------------|----|
| 8  | Spectral diffusion under fast modulation . . . . .                                           | 12 |
| 9  | Optimization Convergence of 4-color Superposition . . . . .                                  | 19 |
| 10 | Experimental details of 2- and 4-color superposition measurements . . . . .                  | 20 |
| 11 | Electronic fine structure model and intersystem crossing mechanism of the $V_{Si}$ . . .     | 21 |
| 12 | Radiative level structure of the $V_{Si}$ in different magnetic field configurations . . . . | 23 |
| 13 | Signatures of ground states interference in $g^{(2)}$ . . . . .                              | 24 |
| 14 | Ramsey pulse sequence . . . . .                                                              | 26 |
| 15 | Single-photon wave-packet from a modulated-two level system . . . . .                        | 28 |
| 16 | Bandwidth expansion via fast Stark shift . . . . .                                           | 29 |
| 17 | Inhomogeneous broadening compensation with dynamic modulation . . . . .                      | 32 |

## 1 Details of the experimental setup

Figures 1 and 2 below present the details of the optical and electrical experimental setups.

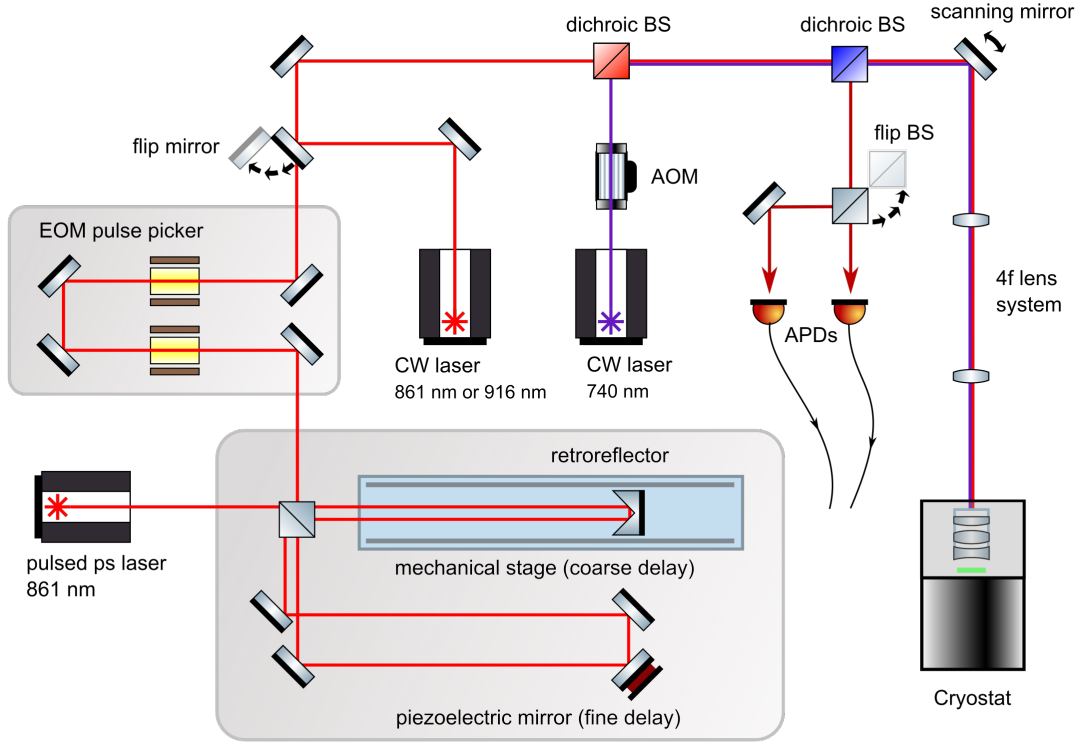

**Supplementary Figure 1: Optical experimental setup.** For PLE measurements, a CW laser (M Squared Lasers) scanned around 861 nm or 916 nm is used to excite the color centers. APDs (Excelitas SPCM-AQRH-14) are used for single photon experiments as well as two-photon correlation (switching between two modes is done with a flip beamsplitter). A scanning confocal setup is used to spatially raster the excitation and detection spots across the sample surface to identify single emitters. For optical pulsed measurements, a picosecond pulsed laser with 80 MHz repetition rate (Spectra Physics, Tsunami) is used. For the Ramsey interference experiment, a combination of a retroreflector on a mechanical stage and a mirror mounted on a piezoelectric crystal produces a pair of pulses with precisely-controlled delay. For the Rabi oscillations experiment requiring only one pulse, one of the paths is blocked. A pair of EOMs (Conoptics, LTA Series EOM) is used for pulse-picking with a 60 dB extinction. Throughout all experiments, above resonant pulsed excitation is used to stabilize the charge of the emitter, produced using a CW laser (MBR) at 740 nm and an AOM. Abbreviations: EOM: electrooptic modulator. AOM: acoustooptic modulator. BS: beamsplitter. CW: continuous wave. APD: avalanche photodiode.

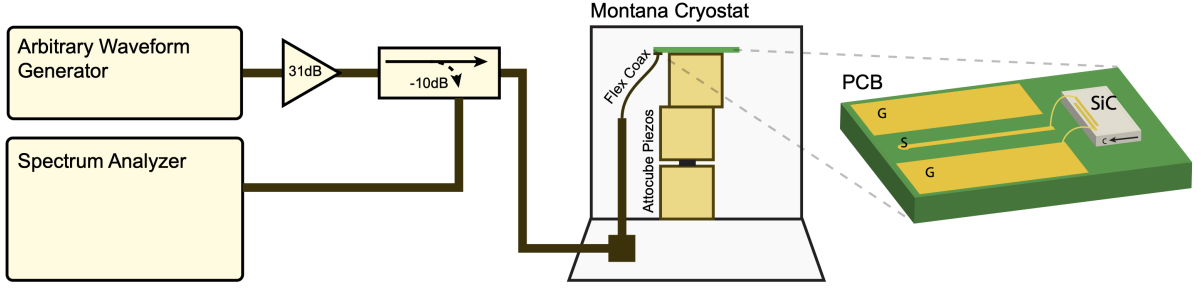

Supplementary Figure 2: **Electrical experimental setup.** The output from an arbitrary waveform generator (Keysight) is amplified (Minicircuits) and delivered to the cryostat via SMA RF cables. The signal is sampled via a -10 dB directional coupler to verify the quality of the amplified signal. Coaxial feedthrough connections allow signal transfer to the inside of the Montana Instruments cryostat. Inside the cryostat, the signal is routed through a flexible coaxial cable to a microwave PCB with a 50 ohm transmission line that terminates open on the 4H-SiC substrate. Three attocube piezoelectric actuators allow for three-axis motion of the sample.

## 2 Additional measurements with DC and AC Stark tuning

### 2.1 Spectral stability and Stark tuning of the negatively charged $k$ - and $h$ - $V_{Si}$ in 4H-SiC

The  $k$ - $V_{Si}$  differs from the  $h$ - $V_{Si}$  in its optical frequency (ZPL at 916 nm compared to 861 nm for  $h$ - $V_{Si}$ ) as well as the zero-field splitting<sup>1</sup>: Compared with the ground (excited) state splitting of  $h$ - $V_{Si}$  of 4.5 MHz (1 GHz), the ground (excited) state splitting in  $k$ - $V_{Si}$  is  $-70$  MHz ( $-1$  GHz)<sup>2,3</sup>. In our experiments, we observe the linewidths of  $k$ - $V_{Si}$  to be about 2-3 times narrower than those of the  $h$ - $V_{Si}$ . As seen in Figs. 4 and 3, the optical transitions of both defects display excellent spectral stability, with optical transitions remaining stable over the course of many hours. From the DC Stark shift measurements of the  $k$ - $V_{Si}$  (Fig. 4d), (assuming the defect position is measured to within  $1 \mu m^3$ ), we deduce a Stark shift of  $3.7 \pm 0.2$  GHz/(MV/m). Thus, the dipole moment of the  $k$ - $V_{Si}$  is within the measurement uncertainty of the value for the dipole moment of the  $h$ - $V_{Si}$ ; this is expected, given the very similar orbital structure of the  $k$ - and  $h$ - $V_{Si}$  defects. We note

that the dipole moment and Stark shift response is reported for the local field, which is calculated via the Lorentz local field approximation<sup>4</sup>. In the Lorentz local field approximation, the relation between the local ( $F$ ) and external ( $E$ ) field is  $F = E(\epsilon + 2)/3$ , where  $\epsilon$  is the dielectric constant of SiC ( $\epsilon_{\text{SiC}} \approx 10$ ). Thus, from experimental considerations, the effective Stark shift of the  $V_{\text{Si}}$  is approximately 4 times higher, since the *local* field experienced by the emitter is 4 times stronger than the *external* field that is obtained from electrostatic simulation.

**2.2 Investigating nonlinearity of Stark shift near 0 V bias** We investigate the “kink” present in the DC Stark shift tuning characteristics near 0 V, to determine whether it is caused by hysteresis. To this end, we scan continuously back and forth around the kink position. We observe that the tuning characteristics are the same for positive and negative voltage ramp, confirming the non-hysteretic nature of the kink (Fig. 5). We attribute it to field rectification by trapped charges, similar to what has been observed in the NV center<sup>5</sup>.

**2.3 Observation of Floquet states in  $h$ - $V_{\text{Si}}$**  Supplementing the Floquet spectrum measurements presented in the Main text for the  $k$ - $V_{\text{Si}}$ , we characterize the properties of the  $h$ - $V_{\text{Si}}$  under rapid modulation. As with the results in the Main text, we find good agreement between experiment and theory (Fig. 6). We note that the  $k$ - $V_{\text{Si}}$  is easier to work with under strong microwave drive, due to its greater resilience to elevated temperatures: for the  $h$ - $V_{\text{Si}}$ , linewidth broadening due to microwave heating of the sample occurs at significantly lower power levels than the  $k$ - $V_{\text{Si}}$ . However,  $h$ - $V_{\text{Si}}$  is still a suitable candidate for fast-modulation application, but care must be taken to use a low-loss microwave architecture, or operate at lower cryogenic temperature.

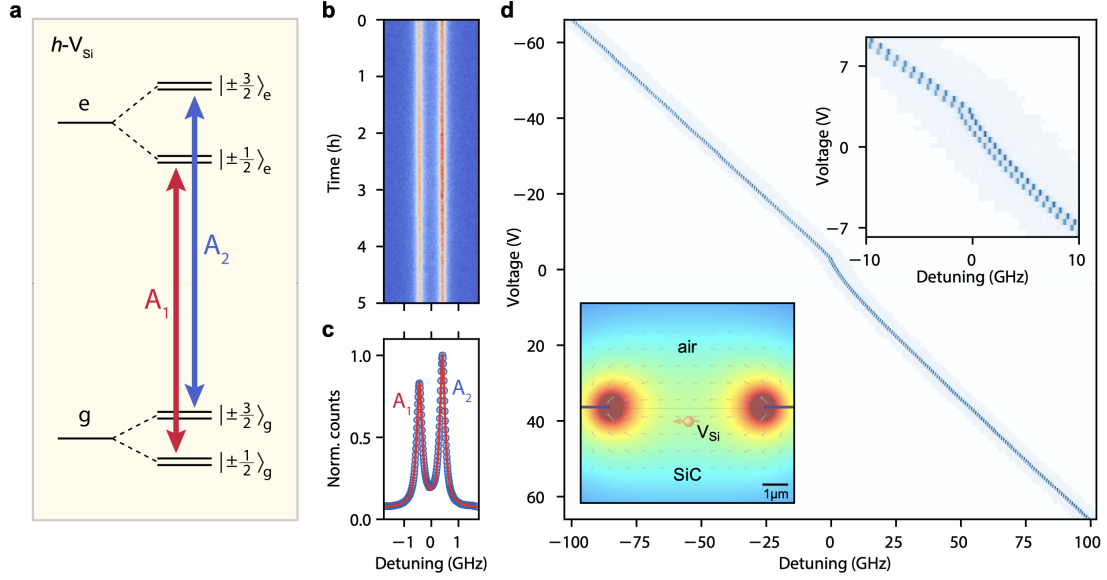

Supplementary Figure 3: **DC Stark tuning characteristics of the  $h$ - $V_{\text{Si}}$ .** **a** The  $h$ - $V_{\text{Si}}$  level structure. **b** Continuous PLE measurement over the course of 5 hours. **c** The intensity of the transitions averaged over the 5-hour acquisition, revealing inhomogeneous linewidths of the  $A_1$  and  $A_2$  transitions to be 259 MHz and 273 MHz, respectively. **d.** The  $V_{\text{Si}}$  frequency is Stark tuned by 200 GHz by applying electric field parallel to the defect's symmetry axis. The detuning is relative to 347.821 THz. Left inset: electrostatic simulation of the field produced by micro-fabricated electrodes. Right inset: the 'kink' observed near bias of 0 V, also seen in the  $k$ - $V_{\text{Si}}$ . A closer investigation of this feature is shown in Fig. 5.

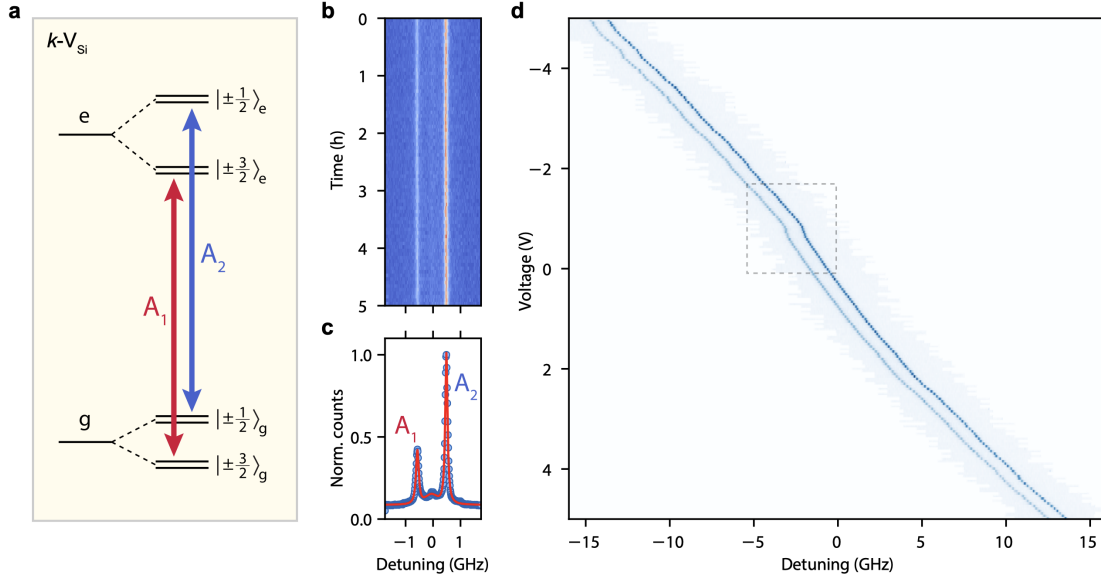

Supplementary Figure 4: **DC Stark tuning characteristics of the  $k$ - $V_{\text{Si}}$**  **a** The  $k$ - $V_{\text{Si}}$  level structure. **b** Continuous PLE measurement over the course of 5 hours. **c** The intensity of the transitions averaged over the 5-hour acquisition, revealing inhomogeneous linewidths of the  $A_1$  and  $A_2$  transitions to be 117 MHz and 100 MHz, respectively. **d** Tuning characteristics of  $V_{\text{Si}}$  for a range of  $\pm 5$  V. The ‘kink’ is observed near 0 V as in the  $h$ - $V_{\text{Si}}$ . The range indicated by the dashed box is investigated in Fig. 5. The detuning is given relative to 326.908 THz.

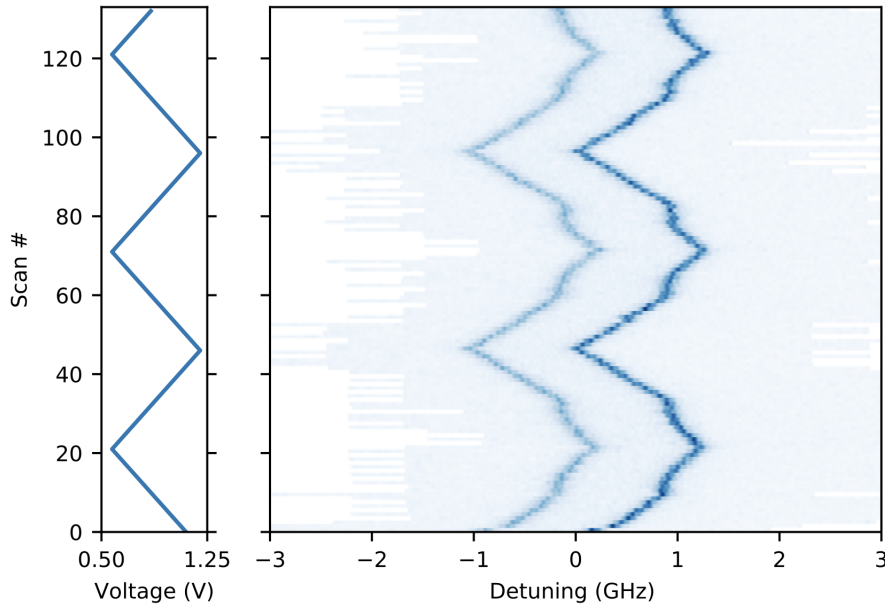

Supplementary Figure 5: **Confirming the non-hysteretic nature of the DC Stark shift near 0 V bias.** As the bias on the electrodes is swept linearly from 0.5 V to 1.25 V and back, it can be seen that the nonlinear behavior is present when scanning in both directions, and thus is not caused by hysteresis. The detuning is given relative to 326.905 THz.

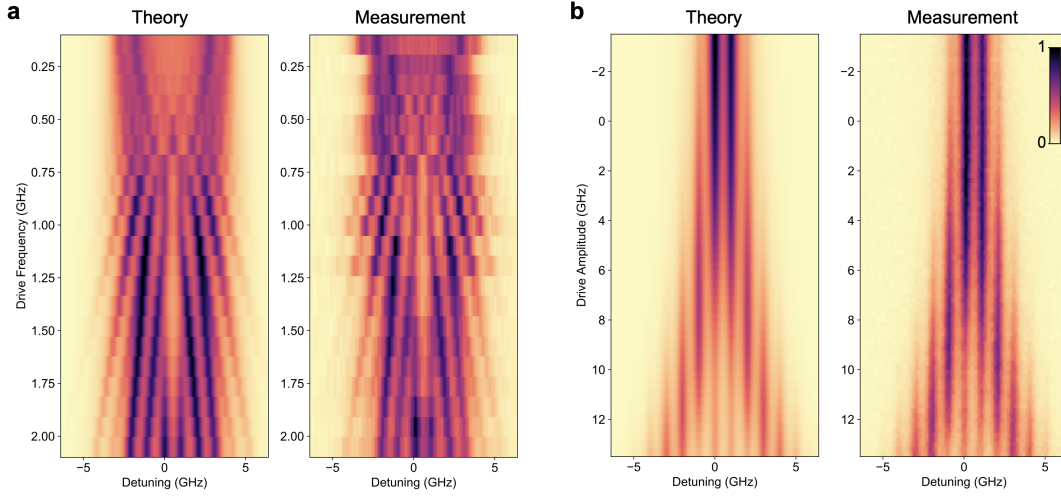

Supplementary Figure 6: **Floquet eigenstates of the  $h$ - $V_{\text{Si}}$  under sinusoidal drive.** **a** Spectral signatures of Floquet states in the  $h$ - $V_{\text{Si}}$  for  $\Delta(t) = A \sin(\Omega t)$  harmonic drive, for swept  $\Omega$  under a fixed amplitude of  $A = 3$  GHz. **b** Spectral signatures of Floquet states with logarithmically swept microwave drive power with fixed  $\Omega/2\pi = 1$  GHz. Color corresponds to the normalized photon counts from the PLE.

**2.4 Large amplitude drive** Figure 7 shows the strongest modulation we could apply at  $\Omega/2\pi = 10$  GHz. The 16 GHz amplitude corresponds to a maximum optical transition slew rate of  $1 \text{ GHz ps}^{-1}$ . At this slew rate, the  $V_{\text{Si}}$  transition traverses its 30 MHz transform-limited linewidth  $1.8 \times 10^5$  times within the optical lifetime of 5.5 ns. Even under such rapid modulation, the optical transitions remain as narrow as in the unmodulated  $V_{\text{Si}}$ , and only three times broader than the transform-limited linewidth.

**2.5 Direct comparison of spectral stability for modulated and unmodulated  $V_{\text{Si}}$**  The narrowest homogeneous linewidth emitters we observe in our sample are around 80-90 MHz, which is only three times broader than transform-limited. Narrower emitters (50-70 MHz) have been previously observed in samples with lower density of defects<sup>2,3,6</sup>. We attribute the larger linewidths

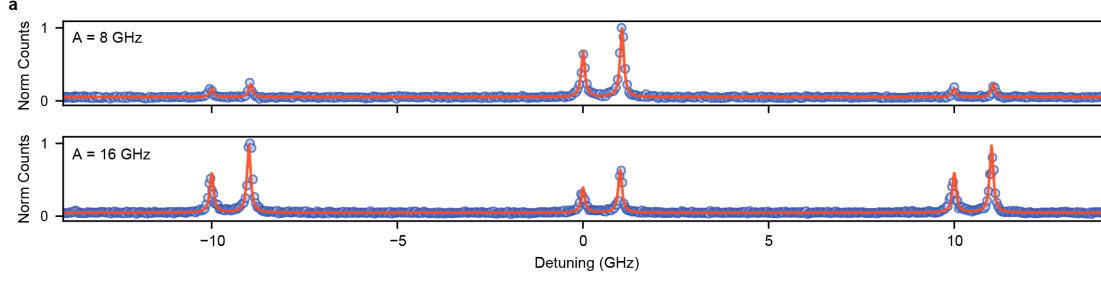

Supplementary Figure 7: **Large amplitude drive of  $k$ -V<sub>Si</sub>** a PLE spectra of a single  $k$ -V<sub>Si</sub> driven at a frequency of 10 GHz and amplitudes of 8 and 16 GHz.

in our sample to a higher electron irradiation dose used to generate defects, which has been shown to induce increased emitter linewidths<sup>2</sup>. As a result of minor spectral diffusion, the narrowest inhomogeneous linewidths we observe are 100 and 102 MHz for the  $k$ - and  $h$ -V<sub>Si</sub>, respectively.

For most potential applications of fast Stark modulation of quantum emitters, it is essential that modulation does not induce additional spectral diffusion. We investigate the effect of spectral diffusion on the  $h$ -V<sub>Si</sub> by collecting the PLE spectra of the same emitter with and without modulation for a duration of 5 hours each, as shown in Fig. 8. The inhomogeneous linewidth of the modulated emitter is nearly identical to that of the unmodulated emitter (105 MHz compared with 102 MHz). We observe that the single modulated emitter linewidth is broader than that of the unmodulated emitter (due to heating effects as experimentally and theoretically described elsewhere<sup>1</sup>). Our data suggests that other than thermal load effects (which can be addressed with improved electrodes design), there are no adverse effects of microwave modulation on the emitter stability.

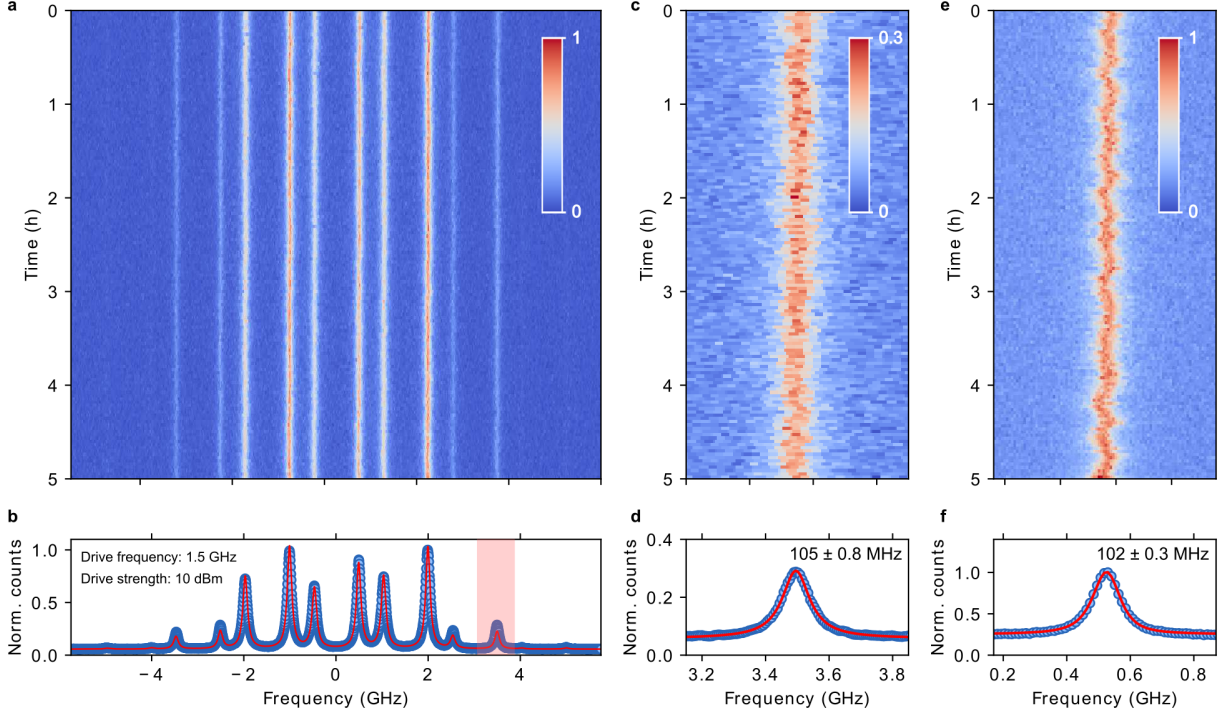

Supplementary Figure 8: **Spectral diffusion under fast modulation.** **a** Continuous PLE measurement over 5 hours of  $h\text{-V}_{\text{Si}}$  under microwave drive of frequency 1.5 GHz and power 10 dBm. **b** Time averaged spectrum. A minor deviation from the theoretical model is seen due to power broadening, present only for the stronger sidebands due to the comparatively stronger coupling to the laser field. **c** A close-up of panel (a) around the Floquet sideband for the A2 transition, identified with a red stripe in panel (b). **d** Lorentzian fit to the time-averaged spectrum of the transition reveals a linewidth of  $105 \pm 0.8$  MHz. **e** Continuous PLE measurement over 5 hours of the A2 transition of the same emitter but without modulation. **f** Lorentzian fit to the time-averaged spectrum of the transition shows a similar inhomogeneous linewidth of  $102 \pm 0.3$  MHz. Frequency is given relative to 347.920 THz

### 3 Scattering matrices for the modulated two-level system

The scattering-matrix formalism can be used to provide analytical expressions for single- and two-photon scattering through the modulated two-level system<sup>7</sup>. The modulated two-level system as an open system can be modeled by considering its interactions with an input channel described by frequency-dependent annihilation operator  $i_\omega$  and an output channel described by a frequency-

dependent annihilation operator  $o_\omega$ . The full open-system Hamiltonian for the modulated two-level system can be expressed as:

$$H(t) = H_{\text{sys}}(t) + \sum_{s \in \{i, o\}} \int_{-\infty}^{\infty} \omega s_\omega^\dagger s_\omega d\omega + \sum_{s \in \{i, o\}} \left( \frac{\gamma_s}{2\pi} \right)^{1/2} \int_{-\infty}^{\infty} (s_\omega^\dagger \sigma + \sigma^\dagger s_\omega) d\omega \quad (1)$$

where  $\gamma_i$  and  $\gamma_o$  are the decay rates associated with the coupling of the modulated two-level system with the input and output channels. The frequency-domain annihilation operators  $i_\omega$  and  $o_\omega$  are assumed to satisfy the bosonic commutation relations  $[i_\omega, i_\nu] = 0$ ,  $[i_\omega, i_\nu^\dagger] = \delta(\omega - \nu)$ ,  $[o_\omega, o_\nu] = 0$ ,  $[o_\omega, o_\nu^\dagger] = \delta(\omega - \nu)$ ,  $[i_\omega, o_\nu] = 0$  and  $[i_\omega, o_\nu^\dagger] = 0$ .

**3.1 Single-photon scattering** The time-domain single-photon scattering matrix,  $S(t, s)$ , which captures the amplitude of producing a photon at time  $t$  in the output waveguide when excited with a photon at time  $s$  in the input waveguide is given by:

$$S(t, s) = -\sqrt{\gamma_i \gamma_o} \langle g | \mathcal{T}[\sigma(t) \sigma^\dagger(s)] | g \rangle \quad (2)$$

where  $\sigma(t)$  and  $\sigma^\dagger(s)$  are the Heisenberg picture operators corresponding to  $\sigma$  and  $\sigma^\dagger$ . While these operators are expressed in the Heisenberg picture with respect to the full Hamiltonian  $H(t)$  (Eq. 1),  $S(t, s)$  can equivalently be computed by considering the Heisenberg picture evolution of  $\sigma$  and  $\sigma^\dagger$  under an effective non-Hermitian Hamiltonian:

$$H_{\text{eff}}(t) = \left( \omega_0 + \Delta(t) - \frac{i\gamma}{2} \right) \sigma^\dagger \sigma \quad (3)$$

where  $\gamma = \gamma_i + \gamma_o$  is the total decay rate of the modulated two-level system. Under this effective Hamiltonian,  $\sigma(t)$  and  $\sigma^\dagger(s)$  can be easily computed:

$$\sigma(t) = \sigma \exp\left(-\frac{\gamma t}{2}\right) \exp\left(-i\omega_0 t - i \int_0^t \Delta(t') dt'\right) \quad (4a)$$

$$\sigma^\dagger(s) = \sigma^\dagger \exp\left(\frac{\gamma s}{2}\right) \exp\left(i\omega_0 s + i \int_0^s \Delta(s') ds'\right) \quad (4b)$$

From Eq. 2 and 4 it follows that:

$$S(t, s) = -\sqrt{\gamma_i \gamma_o} \exp\left[-i \int_s^t \left(\omega_0 - \frac{i\gamma}{2} + \Delta(t')\right) dt'\right] \Theta(t \geq s) \quad (5)$$

The frequency-domain scattering matrix,  $S(\omega, \nu)$ , which captures the amplitude of producing a photon at frequency  $\omega$  in the output waveguide when excited with a photon at frequency  $\nu$  in the input waveguide can be calculated by Fourier-transforming the time-domain scattering matrix  $S(t, s)$ :

$$S(\omega, \nu) = \int_{-\infty}^{\infty} \int_{-\infty}^{\infty} S(t, s) \exp(i(\omega t - \nu s)) \frac{dt ds}{2\pi} \quad (6)$$

Note that if  $\Delta(t)$  averages to 0, then  $\exp\left(-i \int_0^t \Delta(t') dt'\right)$  is periodic in time  $t$  and consequently can be represented as a Fourier series:

$$\exp\left(-i \int_0^t \Delta(t') dt'\right) = \sum_{n=-\infty}^{\infty} \alpha_n \exp(-in\Omega t) \quad (7)$$

From Eqs. 2, 6 and 7, we obtain

$$S(\omega, \nu) = \sum_{p=-\infty}^{\infty} S_p(\nu) \delta(\omega - \nu - p\Omega) \text{ where } S_p(\nu) = - \sum_{m=-\infty}^{\infty} \frac{\sqrt{\gamma_i \gamma_o} \alpha_m^* \alpha_{m+p}}{\gamma/2 + i(\omega_0 + m\Omega - \nu)} \quad (8)$$

The structure of the single-photon scattering matrix indicates that an input photon at frequency  $\nu$  can generate output photons at frequencies  $\nu + p\Omega \forall p \in Z$ . Furthermore,  $S_p(\nu)$  is indicative of the amplitude of the photon at frequency  $\nu + p\Omega$  in the output single-photon state.

**3.2 Two-photon scattering:** Here, we consider the problem of scattering of a monochromatic two-photon state,  $(i_\nu^\dagger)^2 |\text{vac}\rangle$ . The state of the scattered photons in the output channel can be described by its wavefunction  $\psi_{\text{out}}(t, t + \tau; \nu) = \langle \text{vac} | o_t o_{t+\tau} | \psi_{\text{out}}(\nu) \rangle$  where  $o_t$  is the time-domain annihilation operator corresponding to the output channel. In terms of the time-domain two-photon scattering matrix,  $S(t_1, t_2; s_1, s_2)$ ,  $\psi_{\text{out}}(t, t + \tau; \nu)$  is given by:

$$\psi_{\text{out}}(t, t + \tau; \nu) = \int_{-\infty}^{\infty} \int_{-\infty}^{\infty} S(t, t + \tau; s_1, s_2) \exp(-i\nu(s_1 + s_2)) \frac{ds_1 ds_2}{2\pi} \quad (9)$$

Furthermore,  $S(t_1, t_2; s_1, s_2)$  is given by:

$$S(t_1, t_2; s_1, s_2) = \langle g | \mathcal{T} [\sigma(t_1) \sigma(t_2) \sigma^\dagger(s_1) \sigma^\dagger(s_2)] | g \rangle \quad (10)$$

Using Eq. 4, we immediately obtain:

$$S(t_1, t_2; s_1, s_2) = \gamma_i \gamma_o \exp \left[ -i \sum_{i=1}^2 \int_{s_i}^{t_i} \left( \omega_0 - \frac{i\gamma}{2} + \Delta(t') \right) dt' \right] \Theta(t_1 \geq s_1 \geq t_2 \geq s_2) \quad (11)$$

$\Theta(\cdot) = 1$  when its argument is true and is otherwise zero. We have assumed  $t_1 \geq t_2$  and  $s_1 \geq s_2$  since  $S(t_1, t_2; s_1, s_2)$  is symmetric under swap of  $t_1$  with  $t_2$  and  $s_1$  with  $s_2$ . Using Eqs. 11 and 9, we immediately obtain:

$$|\psi_{\text{out}}(t, t + \tau; \nu)|^2 = \gamma_i^2 \gamma_0^2 \left| \sum_{n,m} \frac{\alpha_n^* \alpha_m^* \exp(-i(n+m)\Omega t) (1 - \exp((i(m\Omega - \nu) + \gamma/2)\tau))}{(\gamma/2 + i(\omega_0 + n\Omega - \nu))(\gamma/2 + i(\omega_0 + m\Omega - \nu))} \right|^2 \quad (12)$$

We immediately see that  $|\psi_{\text{out}}(t, t; \nu)|^2 = 0$  — thus, even a modulated two-level system provides perfect photon blockade.

## 4 Floquet engineering

**4.1 Floquet eigenstates** We consider a two-level system with a time-dependent resonant frequency  $\omega_0 + \Delta(t)$ , ground state  $|g\rangle$  and excited state  $|e\rangle$ . Such a system is described by a Hamiltonian:

$$H_{\text{sys}}(t) = (\omega_0 + \Delta(t))\sigma^\dagger \sigma \quad (13)$$

where  $\sigma = |g\rangle \langle e|$  is the de-excitation operator,  $\sigma^\dagger = |e\rangle \langle g|$  is the excitation operator,  $\omega_0$  is the resonant frequency of the two-level system and  $\Delta(t)$  is the periodic modulation in the emitter frequency. We further assume that  $\Delta(t)$  is periodic with fundamental frequency  $\Omega$  with corresponding period  $t_p = 2\pi/\Omega$  and has an average of 0. Accounting for dissipation through the electromagnetic modes coupling to the two-level system, the emission from this system is governed by the effective

Hamiltonian<sup>8,9</sup>:

$$H_{\text{eff}}(t) = H_{\text{sys}}(t) - \frac{i\gamma}{2}\sigma^\dagger\sigma = \left[\omega_0 + \Delta(t) - \frac{i\gamma}{2}\right]\sigma^\dagger\sigma \quad (14)$$

It has been shown that for time-independent systems, the single and two-photon transport properties of quantum systems are determined by the spectral properties of the effective Hamiltonian<sup>9,10</sup>. For periodically modulated systems, it is then necessary to consider the Floquet spectrum of the effective Hamiltonian — the Floquet states  $|\phi(t)\rangle$  and the corresponding Floquet eigenvalues  $\varepsilon$  are defined as the solution of the following eigenvalue problem:

$$\left[H_{\text{eff}}(t) - i\frac{d}{dt}\right]|\phi(t)\rangle = \varepsilon|\phi(t)\rangle \quad (15)$$

with the periodic boundary condition,  $|\phi(t + t_p)\rangle = |\phi(t)\rangle$ , imposed on  $|\phi(t)\rangle$ . The Floquet states and Floquet energies for the Hamiltonian in Eq. 14 can be computed analytically and are given by:

$$|\phi_0(t)\rangle = |g\rangle, \varepsilon_0 = 0 \text{ and } |\phi_1(t)\rangle = \exp\left[-i\int_0^t \Delta(\tau)d\tau\right]|e\rangle, \varepsilon_1 = \omega_0 - \frac{i\gamma}{2} \quad (16)$$

Since the periodic signal  $\Delta(t)$  averages out to 0 over its period, it immediately follows that  $\phi(t)$  is periodic in time with period  $t_p$ . Consequently, it is possible to expand  $\exp(-i\phi(t))$  into a Fourier series:

$$\exp(-i\phi(t)) = \sum_{n=-\infty}^{\infty} \alpha_n \exp(-in\Omega t) \quad (17)$$

The Fourier coefficients  $\alpha_n$  govern the output state of the photons emitted by such a two-level system when excited with a coherent state. Engineering the temporal shape of the modulation  $\Delta(t)$  can be used to design the coefficients  $\alpha_n$  and consequently control the properties of the photons emitted by the two-level system.

**4.2 Floquet state engineering** To optimize single photon superposition states, we need to optimize over the single photon scattering matrix. Under fast modulation, when the input frequency  $\nu$  is resonant with the sideband at  $\omega_0 + m\Omega$ , it follows that:

$$S_p(\nu) \approx -\frac{\sqrt{\gamma_i \gamma_o} \alpha_m^* \alpha_{m+p}}{\gamma/2 + i(\omega_0 + m\Omega - \nu)} \quad (18)$$

It can be seen from equation (7) that in this regime total transmission  $T(\nu) \sim |\alpha_m|^2$ . Therefore we can optimize over the  $a_m$ s, given by the Fourier series components of  $e^{-i \int_0^t \Delta\omega(\tau) d\tau}$ .

Here we show the optimization process used to generate the 4-color superposition state given in Figure 4 in the main text. Fig. 9a shows the mean squared error of the frequency distribution per iteration of the BFGS algorithm, and Fig. 9b shows the constituent frequency decomposition at each iteration. As the optimizer is initialized to 0 microwave amplitude, the resonant frequency initially contains all optical power. As the state is optimized, this power drops and the desired frequency components approach the goal distribution.

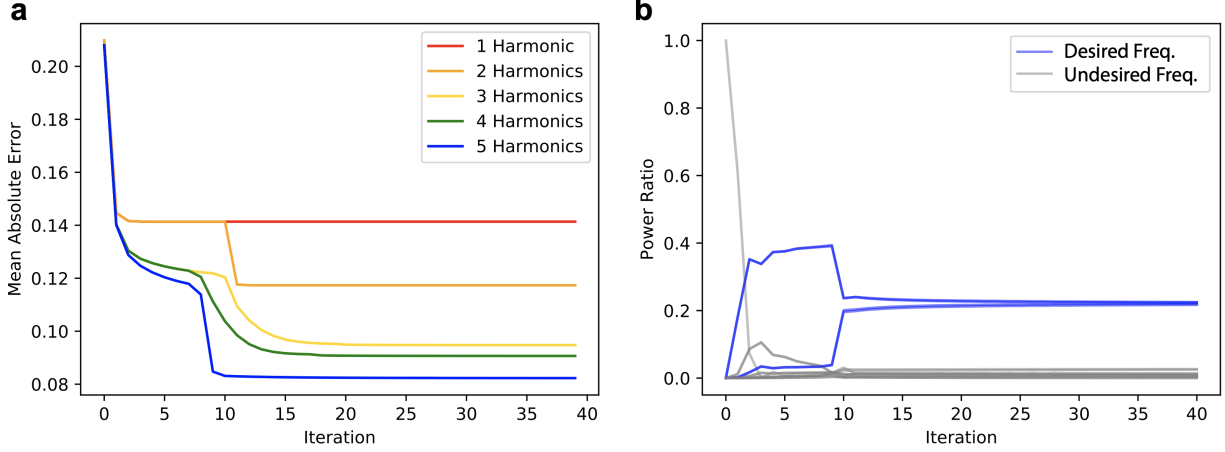

Supplementary Figure 9: Optimization Convergence of 4-color Superposition. **a** Mean absolute error over 40 BFGS iterations with 1 to 5 harmonics included in the optimization. **b** Spectral content of 5 harmonic optimization over the 40 BFGS iterations. Blue denotes the 4 non-zero frequencies in the optimization target. Note that only 2 non-overlapping blue lines are visible as in this case the optimization was symmetric.

**4.3 Realizable spectra** From the floquet excited state phase  $\exp\left(-i \int_0^t \Delta(\tau) d\tau\right)$ , we see that we can apply any time-dependent phase that is differentiable through a corresponding modulation  $\Delta(t)$ . This time-dependent phase determines the realizable spectra in the following ways.

In the regime of short pulsed excitations, the modulated spectra achievable will be broadened by the linewidth of the emitter. Additionally, in this regime synchronization between the excitation and modulation is necessary to generate identical photons. This requirement can be lifted if the period of modulation is much shorter than the optical lifetime of the emitter.

In the regime of long excitations, tending to continuous-wave, the spectrum can be shaped through modulation and through the shaping of the excitation pulse. In this regime the set of achievable spectra is no longer affected by linewidth broadening. Any photon spectrum whose

corresponding temporal phase is differentiable can be achieved through modulation, and the temporal amplitude can be shaped arbitrarily by the excitation pulse.

**4.4 Experimental details of photon color-superpositions** To experimentally verify the Floquet engineering protocol, we applied the microwave drives shown in Figure 10 and measured the PLE spectra shown in the main text Figure 4.

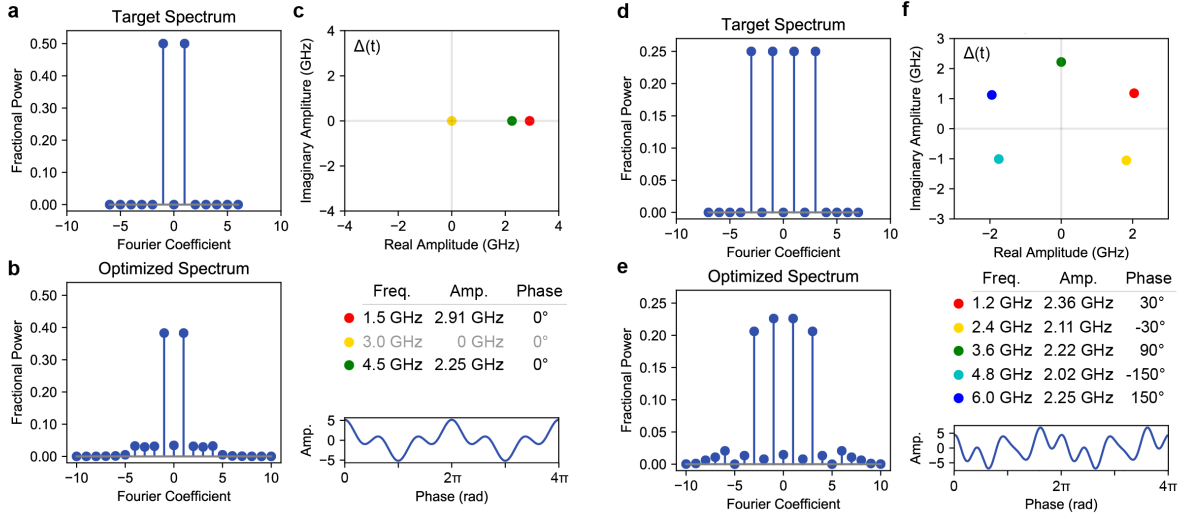

Supplementary Figure 10: Experimental details of 2- and 4-color superposition measurements. **a** Target spectrum for 2-color superposition. **b** Optimal spectrum using 3 microwave harmonics. **c** Optimal drive conditions for experiment in Figure 4. **d-f** Correspond one to one to a-c but for a 4-color superposition with 5 microwave harmonics.

## 5 Signature of ground state interference in $g^{(2)}(\tau)$

**5.1 Theoretical model for the  $h$ - $V_{Si}$  structure** The  $h$ - $V_{Si}$  Hamiltonian is given as  $H = H_{ZFS} + H_Z + H_d$  in terms of zero field splitting (ZFS)  $H_{ZFS} = \sum_{i=g,e} D_i(S_{i,z}^2 - 5/4)$  and Zeeman interaction  $H_z = \sum_{i=g,e} g\mu_B \vec{B} \cdot \vec{S}_i / \hbar$  spin Hamiltonians<sup>11</sup> in which  $\vec{S}_i$  are the well known spin-3/2 operators in each ground ( $g$ ) and excited ( $e$ ) state subspaces. The optical drive between the ground

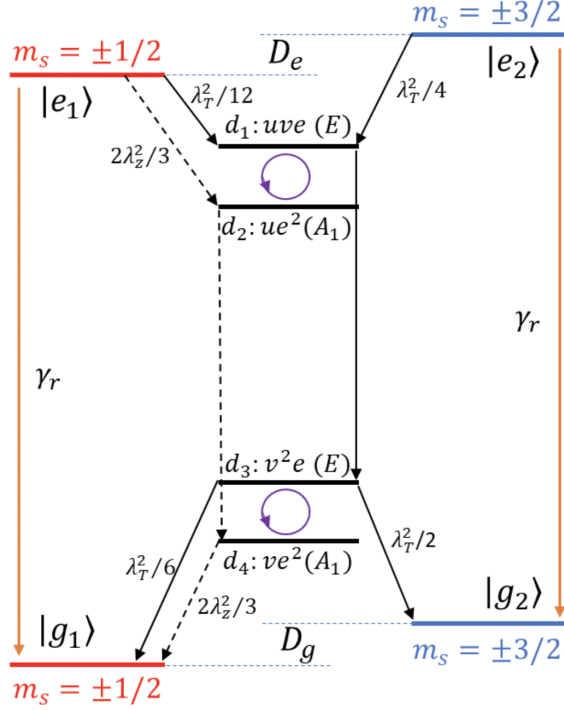

Supplementary Figure 11: Electronic fine structure model and intersystem crossing mechanism of the  $V_{Si}$ . The radiative decay rates for both spin-3/2 and -1/2 channels are labeled as  $\gamma_r$ . The ground and excited state ZFS are given by  $D_g$  and  $D_e$ , respectively. Additional potential spin relaxation processes between allowed doublets (via spin-orbit coupling) are shown by circular arrows. Dashed and solid black arrows correspond to ISC channels assisted by the longitudinal and orthogonal components (with respect to the c-axis) of the spin-orbit coupling and optical emission polarization.

and the excited states is represented by  $H_d = \sum_i \omega (a e^{-i\omega_d t} |e_i\rangle \langle g_i| + \text{h.c.})$  for a laser of frequency  $\omega_d$  and amplitude  $\Omega$  (Rabi frequency). All radiative and nonradiative (intersystem crossing) decay processes of the  $V_{Si}$  defect are represented by the Lindblad super-operators and shown in Fig. 11. The final Hamiltonian is constructed in the 12 Hilbert space spanned by four excited, four ground, and four metastable states shown in Fig. 11 that are previously determined by the electronic structure calculations and group theoretical analysis<sup>12</sup>.

All four ( $d_1 - d_4$ ) metastable states with  $ve^2$  ( $A_1$ ),  $v^2e$  (E),  $ue^2$  ( $A_1$ ), and  $uve$  (E) orbital configurations (symmetry), shown in Fig. 11, form the intersystem crossing mechanism of this defect and responsible for the spin polarization. Due to their equal transition moments, both spin  $m_s = \pm 3/2$  ( $|e_2\rangle \rightarrow |g_2\rangle$ ) and  $m_s = \pm 1/2$  ( $|e_1\rangle \rightarrow |g_1\rangle$ ) radiative decay channels have the same rate  $\gamma_r$ . The general relationship between each non-radiative decay channel, within the same doublet orbital manifold, can be obtained by the phonon assisted direct spin-orbit coupling matrix elements, in the form of  $\frac{2\pi}{\hbar} \left| \langle \psi_{g,e} | \sum_j \lambda_z l_j^z s_j^z + \lambda_T l_j^{x,y} s_j^{x,y} | \psi_{d_1-d_4} \rangle \right|^2$  in the symmetry adapted wave-function basis of the  $j = 5$  active electrons of this defect center<sup>12</sup>. Therefore, the symmetry allowed nonradiative decay channels into and out of all the metastable states are identified by their corresponding spin orbit coupling coefficients  $\lambda_z$  (parallel to the  $c$ -axis) and  $\lambda_T$  (perpendicular to the  $c$ -axis) in Fig. 11. We note that, even though we use our 12-dimensional extended Hamiltonian for  $g^{(2)}(\tau)$  calculations here, in the presence of fast spin relaxation among  $d_1 \leftrightarrow d_2$  and  $d_3 \leftrightarrow d_4$  doublet states, the electronic fine structure of the  $V_{Si}$  can be reduced to earlier simplified models<sup>2,3</sup> that involves only two metastable doublets instead of the four used here. Furthermore, here we assume the decay from upper to lower doublet states is due to emission of photons. Although these transitions can also be assisted by generally slower phonon processes, this does not affect our results here as both possibilities are indirectly taken into account under the overall lifetime of the metastable doublet states found here. Further studies in the future resolving the detailed breakdown of the metastable state lifetimes may allow for the identification of the underlying dominant decay process between the doublets.

Figure 12 shows the effect on the optical level structure of the defect of the two magnetic

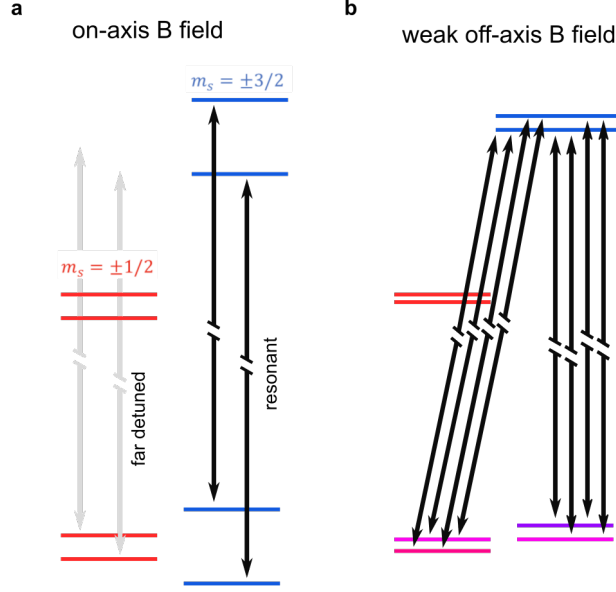

Supplementary Figure 12: Radiative level structure of the  $V_{Si}$  in different magnetic field configurations. **a** In a magnetic field aligned with the symmetry axis (*i.e.*  $B_x = 0$ ), the optical transitions are spin-conserving. When resonantly addressing the  $\pm 3/2$  transitions, the  $\pm 1/2$  transitions are far detuned and are not excited. **b** When a low off-axis magnetic field is applied, the ground state spins are hybridized. The excited  $\pm 3/2$  states, however, remain unhybridized due to the much larger excited state ZFS. The non-uniform hybridization is indicated in purple for illustrative purposes. The resulting optical level structure comprises total of 8 optical transitions varying only slightly (order of 10 MHz) in frequency. Crucially, unlike in the axial field case shown in (a), ground states are interacting via spin-non-conserving optical transitions.

field configurations studied in this work. For all experiments other than the  $g^{(2)}(\tau)$  measurements, the axial  $B$  field configuration is used (shown in Fig. 12a). For  $g^{(2)}(\tau)$ , however, this configuration cannot be used, as the intersystem crossing channel would depopulate the resonantly pumped optical transition and cause the emitter to go into a dark state. While an rf-magnetic field can be used to induce spin mixing in the ground state, such an approach would introduce a time-dependent term in the Hamiltonian in addition to the studied Stark shift modulation; This would potentially compromise the integrity of the experiment, which aims to isolate the effect of Stark modulation on the two-photon scattering properties. As such, a low, off-axis B-field is applied to allow all

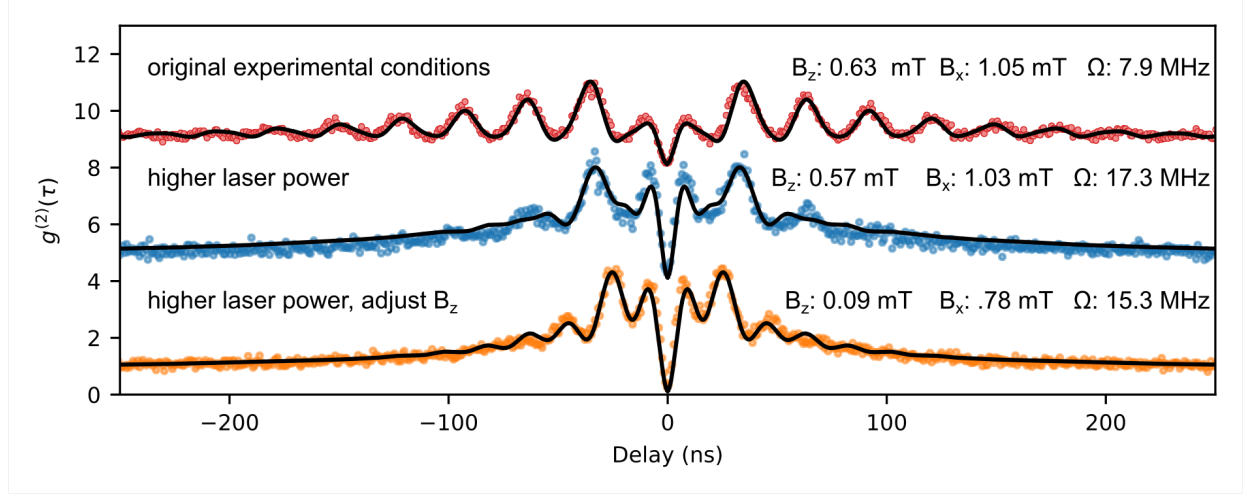

Supplementary Figure 13: Signatures of ground states interference in  $g^{(2)}$ . Top dataset is used to extract the three unknown rates of the  $V_{Si}$  described in the text. Then, a higher laser power is applied, and a fit to the model is obtained using the external parameters  $B_z, B_x, \Omega$ , whose resulting values are shown in the second dataset. Then, with laser power held at the higher level, axial magnetic field was adjusted, and the measurement was repeated (bottom dataset)

states in the ground manifold to couple to the  $\pm 3/2$  excited state subspace.

**5.2 Observation of interference of multiple ground states via  $g^{(2)}$ .** Using our full extended 12-dimensional Hamiltonian, and the quantum regression theorem<sup>10</sup> we numerically evaluate  $g^{(2)}(\tau)$  and fit it to the experimental data using three unknown  $V_{Si}$  rates (radiative branching ratio, metastable state lifetime, and doublet mixing rate) and well three external parameters (the laser drive strength and the axial and transverse magnetic field strengths). The numerical fit overlaid with experimental data is shown in the top dataset in Fig. 13. The branching ratio, metastable lifetime, and doublet mixing are fit to be 0.75, 690 ns, and 5.8 ns, respectively.

We then proceed to change the laser drive power and magnetic field strength, and observe a change in the ground state interference pattern. At higher laser power, we observe a drop in

the coherence at longer timescales: This is predicted by the model, as it causes a faster rate of population transfer to the metastable state, where incoherent phonon interactions destroy the spin coherence. Then, keeping the same laser power we adjust the external magnet to decrease  $B_z$ . As expected, we observe a change in the period of oscillations, which arises from the fine splitting between the ground states. Our numerical model (fit with the three aforementioned “external” parameters) agrees well with the experimental data. For a targeted study of ground state interference in  $g^{(2)}(\tau)$ , integration of rf-B-field delivery to the sample would enable independent verification of the ground state splitting via optically-detected magnetic resonance, and thus permit a fitting with fewer free parameters.

## 6 Ramsey interference experiment

**6.1 Experimental details** Figure 1 shows the experimental setup used to investigate Ramsey interference. Not pictured in the diagram is an additional tunable band pass filter (Semrock) placed before the single photon detector, which is used to increase the rejection ratio of the resonant laser; as well as a permanent magnet mounted to produce approximately 20mT field along the symmetry axis of the defect, in order to polarize the ground state manifold. Thermal and acoustic isolation of the experimental setup use to produce the pulse sequence enables high stability of the fine interpulse delay, with drift rates of approximately 1 fs per hour. The data presented is corrected for this residual drift. The 6 MHz repetition rate pulse sequence is produced with a delay generator (Stanford Research Systems, DG645), triggered by the intrinsic laser repetition rate (80 MHz). The pulse sequence is shown in Fig. 14.

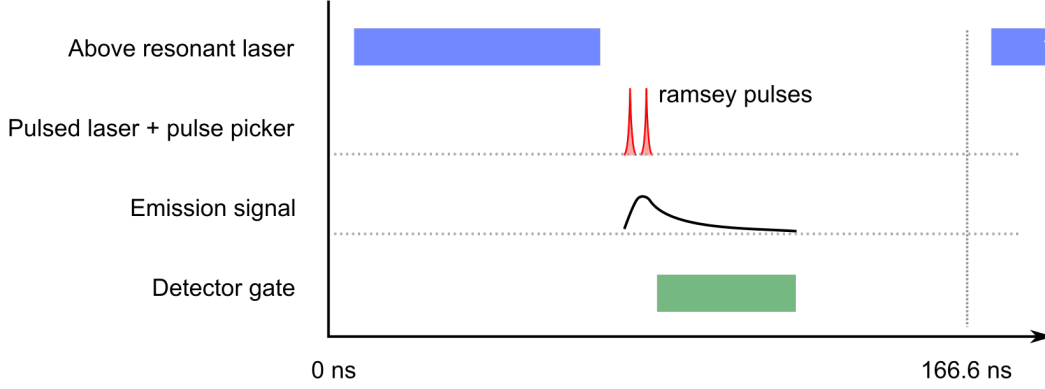

Supplementary Figure 14: Ramsey pulse sequence. First, an above resonant pulse initializes the emitter into an equal mixture ground state. A pair of 3 ps pulses (x-axis not to scale) manipulate the emitter orbital state. The single photon detector is gated to only detect the transient signal from the  $V_{Si}$  (optical lifetime 6 ns).

**6.2 Ramsey interference contrast in a modulated TLS** For an unmodulated TLS excited with two  $\pi/2$  pulses delayed by a time  $t_{delay}$  where  $t_{delay} \ll 1/\gamma$ , the Ramsey interference pattern is given by

$$I_R(t_{delay}) = \frac{1}{2} + \frac{1}{2} \cdot \cos(\omega_0 \cdot t_{delay}). \quad (19)$$

A sinusoidally modulated TLS experiences an additional phase due to its modulation,

$$A \int_0^{t_{delay}} \cos(\Omega t + \phi) dt = \frac{A}{\Omega} [\sin(\Omega t_{delay} + \phi) - \sin(\phi)], \quad (20)$$

where  $\phi$  is the microwave phase relative to the Ramsey pulses.

For modulation frequencies that are not multiples of  $1/t_{delay}$ , the time-averaged Ramsey contrast due to this phase is

$$I_R(t_{delay}, A, \Omega) = \frac{1}{2} + \frac{1}{2} \cdot \frac{1}{2\pi} \int_0^{2\pi} \cos\left(\omega_0 \cdot t_{delay} + \frac{A}{\Omega} [\sin(\Omega t_{delay} + \phi) - \sin(\phi)]\right) d\phi, \quad (21)$$

which can be simplified to

$$I_R(t_{\text{delay}}, A, \Omega) = \frac{1}{2} + \frac{1}{2} \cdot \cos(\omega_0 \cdot t_{\text{delay}}) \cdot J_0\left(\frac{2A}{\Omega} \sin\left(\frac{\Omega \cdot t_{\text{delay}}}{2}\right)\right). \quad (22)$$

## 7 Spontaneous decay of a spectrally-optimized photon

To compute the state of the emitted photon when the modulated two-level system is driven by a short laser pulse  $\Omega(t)$ , we incorporate the laser drive into the effective Hamiltonian to obtain:

$$H_{\text{eff}}(t) = \left(\omega_0 + \Delta(t) - \frac{i\gamma}{2}\right) \sigma^\dagger \sigma + \Omega(t) (\sigma \exp(i\omega_L t) + \sigma^\dagger \exp(-i\omega_L t)) \quad (23)$$

Assuming that the two-level system emits into an optical mode with annihilation operator  $a_\omega$  with decay rate  $\gamma$  and that at  $t = 0$  the optical mode is in the vacuum state and the two-level system is in the ground state, the spectrum of the emitted single photon at time  $t_f$ ,  $\psi(\omega, t_f)$ , is given by<sup>8</sup>:

$$\psi(\omega, t_f) = -i\sqrt{\frac{\gamma}{2\pi}} \int_0^{t_f} \langle g | U_{\text{eff}}(t_f, t) \sigma U_{\text{eff}}(t, 0) | g \rangle \exp(i\omega t) dt \quad (24)$$

The numerical calculation of photons emitted spontaneously in two- and four-color is shown in Fig. 15.

## 8 Proposed applications for rapidly modulated quantum emitters

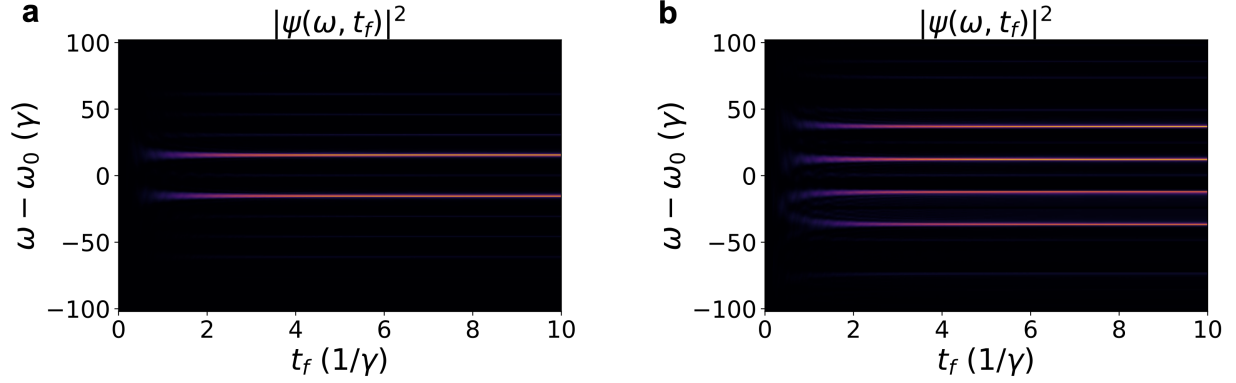

Supplementary Figure 15: Single-photon wave-packet emitted at time  $t_f$  for a modulated-two level system with the modulation  $\Delta(t)$  being designed for **a** 2-color superposition (**b** 4-color superposition) when the two-level system is driven by a short Gaussian laser pulse.

**8.1 Aperiodic modulation for bandwidth expansion** Fast periodic modulation of a TLS restricts the photon to a discrete, comb-like spectrum, a restriction that is lifted for aperiodic modulation. We explore numerically an application of aperiodic modulation to bandwidth expansion of single photons, enabled by the high slew rate attainable with Stark shift modulation. The approach is illustrated in Fig. 16. In the absence of modulation, the TLS emits narrowband Lorentzian photons (Fig. 16a). By frequency-chirping the TLS in the process of photon emission (Fig. 16b), it is possible to match the spectral composition of the single-photon wavepacket to that of a much broader Gaussian pulse (Fig. 16c) (see Supplementary Information). However, the emitted photon is chirped (Fig. 16d). Through dispersion correction (*e.g.*, by passing through a chirped fiber Bragg grating<sup>13</sup>), the photon can be converted into a short, nearly-Gaussian pulse (Fig. 16e,f). Using the  $V_{\text{Si}}$  tuning parameters obtained in experiment, we find that bandwidth expansion by three orders of magnitude is achievable. Such bandwidth control is particularly beneficial for connecting quantum nodes that operate at very different timescales, such as quantum dots, superconducting qubits,

and rare earth ions. Temporal compression would also ease the power requirements for quantum frequency conversion in a waveguide.

The dispersion correction required for the example given in figure 16, a group delay difference of 19ns across a 100 GHz bandwidth, is likely achievable but is larger than has been demonstrated. Linear chirped fiber bragg gratings can achieve close to this amount of dispersion

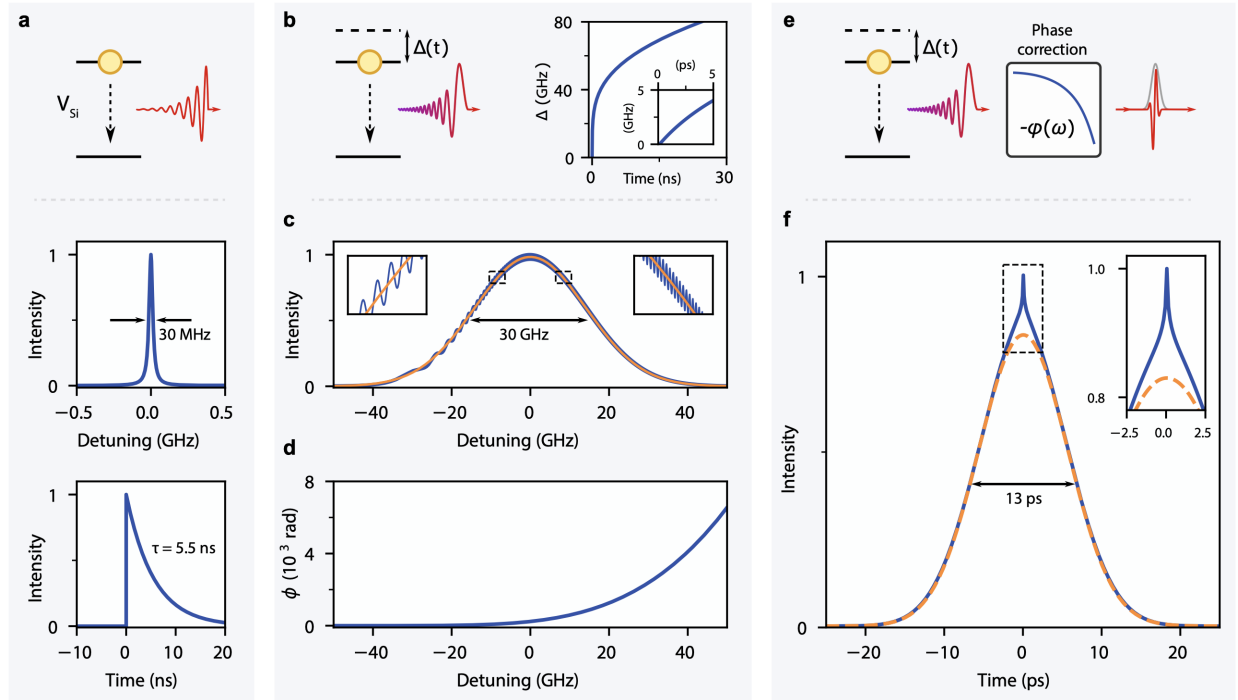

Supplementary Figure 16: **Bandwidth expansion via fast Stark shift** **a** A photon emitted spontaneously from an unmodulated  $V_{Si}$  possesses a Lorentzian spectrum with a lifetime-limited linewidth of 30 MHz and an exponential temporal envelope. **b** An appropriately-chosen  $\Delta(t)$  (not exceeding the maximum demonstrated slew rate of  $1 \text{ GHz ps}^{-1}$ ) applied to the  $V_{Si}$  initially in the excited state causes the  $V_{Si}$  to emit a chirped photon with a broad, near-Gaussian spectrum, as shown in **c**. **d** Although the frequency composition of the emission is Gaussian, the pulse is chirped, as seen from the relative phases of the constituent frequencies. **e** The chirped photon can be phase-corrected by dispersion engineering to be transformed into a short pulse with a near-Gaussian temporal profile. **f** The resulting dispersion-corrected pulse, now only 13 ps long, deviates only slightly at its center from the Gaussian profile, a nonideality that originates from the fine oscillations in the spectrum, shown in the insets in **c**.

– R. Woodward et al.<sup>13</sup> achieve a 4ns group delay difference across a 600 GHz bandwidth. This work uses a 400mm linearly chirped fiber, so it would be conceivable to fabricate a larger fiber to achieve the desired dispersion. However, if the bragg grating were chirped quadratically instead of linearly, an immensely greater dispersion compensation can be achieved in the same length. While this would introduce cubic dispersion, it may be possible to engineer the bragg grating to compensate. By using ultraslow-light techniques<sup>14</sup>, it may even be possible to integrate the dispersion compensation on-chip with high quality photonics. Using a quadratically-chirped silicon carbide grating, the minimum length to accrue the phase difference in Fig. 16d is only 200um. In practice, the grating may need to be larger to prevent scattering losses and to maintain a bandgap, but this can be significantly aided by a slow-light design. Additionally, the compactness and dispersion can be further enhanced by using a cavity arrangement<sup>15</sup>.

To find the optimum  $\Delta(t)$  necessary to generate bandwidth-expanded photon with a Gaussian power-spectrum composition, the output photon spectrum from the aperiodically driven system must be calculated for a given  $\Delta(t)$ , and then numerical optimization of  $\Delta(t)$  must be performed. The spectral composition of the emitted photon is given by the Fourier transform of the photon's temporal amplitude, which is given by  $-i\sqrt{\gamma}\sigma(t)$  (from input-output formalism<sup>16</sup>). Assuming the emitter is prepared in the excited state at time  $t = 0$ , the photon shape in time is thus<sup>8</sup>

$$s(t) = \langle e | U_{\text{eff}}(t, 0) | e \rangle, \quad (25)$$

where  $U_{\text{eff}}$  is the propagator corresponding to the effective Hamiltonian. The complex spectrum of

the photon is obtained by taking the Fourier transform of  $s(t)$ . We optimize  $\Delta(t)$  via BFGS using the  $f_n(t) = a_n t^{1/n}$  functions as the basis, while constraining the maximum slew-rate to not exceed the experimentally-demonstrated value.

**8.2 Inhomogeneous broadening compensation in strongly coupled cavity QED** An important challenge in cavity QED with multiple emitters is that the resonant frequencies of the emitters can be significantly different from each other, forbidding a collective strong interaction between the emitters and a cavity mode. Application of a time-dependent frequency modulation on the emitters can allow for a strong collective interaction from emitters with vastly different frequencies. In order to illustrate this theoretically, we consider  $N$  emitters with lowering operators  $\sigma_1, \sigma_2 \dots \sigma_N$  coupling to a cavity mode with annihilation operator  $a$  with coupling strength  $g$ . The emitter frequencies, relative to the cavity resonance, are denoted by  $\Delta_1, \Delta_2 \dots \Delta_N$  and a time-dependent modulation  $\delta(t)$  is applied uniformly on all the emitters. This system is modeled by the time-dependent Hamiltonian  $H(t)$ :

$$H(t) = \sum_{i=1}^N \left[ (\delta(t) + \Delta_i) \sigma_i^\dagger \sigma_i + g(a \sigma_i^\dagger + \sigma_i a^\dagger) \right] \quad (26)$$

We consider a regime in which the broadening in  $\Delta_i$  is much larger than  $g$ :  $\text{stddev}[\Delta_i] \sim 10g$  — consequently, in the absence of modulation only one of the emitters can significantly interact with the cavity mode. To design the pulse  $\delta(t)$  that would enable strong interactions between the emitters and the cavity mode, we computationally minimize the distance between the propagator corresponding to one period of  $H(t)$ ,  $U_{\text{pulsed}}$ , and the propagator  $U_{\text{target}}$  corresponding of the target

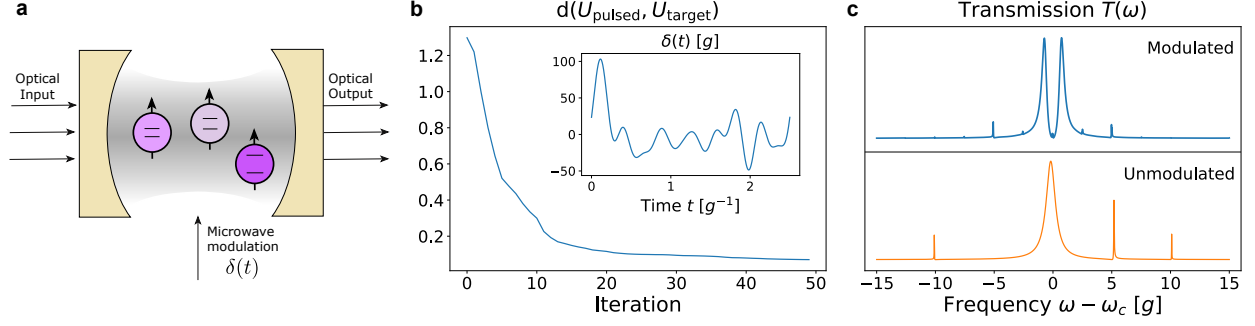

Supplementary Figure 17: **Inhomogeneous broadening compensation with dynamic modulation:** **a** A schematic depiction of a multi-emitter cavity QED system with inhomogeneous broadening and a microwave modulation  $\delta(t)$  uniformly applied to all the emitters. **b** The distance between the propagator corresponding to the modulated multi-emitter cavity QED system and the target propagator as a function of the optimization iteration, with the finally obtained pulse shown as an inset. **c** The transmission spectrum of the 3-emitter system with and without the modulation. Application of the modulation induces strong interactions between the emitters and the cavity mode as is evidenced by the polaritonic splitting visible in the transmission spectrum of the modulated system (absent for the unmodulated system because of inhomogeneous broadening).

Hamiltonian  $H_{\text{target}} = g \sum_{i=1}^N (a\sigma_i^\dagger + \sigma_i a^\dagger)$ . The distance measure we choose in our calculations is that induced from a Frobenius norm — more specifically, the distance between two operators  $U_1$  and  $U_2$  is calculated as  $d(U_1, U_2) = \text{Tr}[(U_1 - U_2)^\dagger (U_1 - U_2)] / \text{dim}(\mathcal{H})$  where  $\text{dim}(\mathcal{H})$  is the dimensionality of the Hilbert space being considered. We restrict ourselves to the single-excitation subspace of the multi-emitter cavity QED system and solve the resulting optimization problem the L-BFGS optimizer. Fig. 17b shows the distance between the two propagators as a function of the optimization iteration — the finally optimized pulse  $\delta(t)$  is shown as an inset. Fig. 17c shows the transmission spectrum of the multi-emitter cavity QED system with and without the applied modulation — in the absence of the modulation, we see distinctive peaks corresponding to the uncoupled cavity mode and the emitters, while in the presence of modulation the emitters strongly interact with the cavity mode as is evidenced by the polaritonic splitting visible in the transmission spectrum.

## 9 References

1. Udvarhelyi, P. *et al.* Vibronic states and their effect on the temperature and strain dependence of silicon-vacancy qubits in 4 h-si c. *Phys. Rev. Appl.* **13**, 054017 (2020).
2. Nagy, R. *et al.* High-fidelity spin and optical control of single silicon-vacancy centres in silicon carbide. *Nat. Commun.* **10**, 1–8 (2019).
3. Banks, H. B. *et al.* Resonant optical spin initialization and readout of single silicon vacancies in 4H-SiC. *Phys. Rev. Applied* **11**, 024013 (2019).
4. Tamarat, P. *et al.* Stark shift control of single optical centers in diamond. *Phys. Rev. Lett.* **97**, 083002 (2006).
5. Bassett, L., Heremans, F., Yale, C., Buckley, B. & Awschalom, D. Electrical tuning of single nitrogen-vacancy center optical transitions enhanced by photoinduced fields. *Phys. Rev. Lett.* **107**, 266403 (2011).
6. Morioka, N. *et al.* Spin-controlled generation of indistinguishable and distinguishable photons from silicon vacancy centres in silicon carbide. *Nat. Commun.* **11**, 1–8 (2020).
7. Trivedi, R., White, A., Fan, S. & Vučković, J. Analytic and geometric properties of scattering from periodically modulated quantum-optical systems. *arXiv preprint arXiv:2003.10673* (2020).
8. Trivedi, R., Fischer, K., Xu, S., Fan, S. & Vuckovic, J. Few-photon scattering and emission from low-dimensional quantum systems. *Phys. Rev. B* **98**, 144112 (2018).

9. Xu, S. & Fan, S. Input-output formalism for few-photon transport: A systematic treatment beyond two photons. *Phys. Rev. A* **91**, 043845 (2015).
10. Trivedi, R., Radulaski, M., Fischer, K. A., Fan, S. & Vučković, J. Photon blockade in weakly driven cavity quantum electrodynamics systems with many emitters. *Phys. Rev. Lett.* **122**, 243602 (2019).
11. Soykal, Ö. & Reinecke, T. L. Quantum metrology with a single spin-3 2 defect in silicon carbide. *Phys. Rev. B* **95**, 081405 (2017).
12. Soykal, Ö., Dev, P. & Economou, S. E. Silicon vacancy center in 4H-sic: Electronic structure and spin-photon interfaces. *Phys. Rev. B* **93**, 081207 (2016).
13. Woodward, R. *et al.* Fiber grating compression of giant-chirped nanosecond pulses from an ultra-long nanotube mode-locked fiber laser. *Optics Lett.* **40**, 387–390 (2015).
14. Notomi, M., Kuramochi, E. & Tanabe, T. Large-scale arrays of ultrahigh-q coupled nanocavities. *Nat. Photonics* **2**, 741 (2008).
15. Yu, S.-P., Jung, H., Briles, T. C., Srinivasan, K. & Papp, S. B. Photonic-crystal-reflector nanoresonators for kerr-frequency combs. *ACS Photonics* **6**, 2083–2089 (2019).
16. Gardiner, C. W. & Collett, M. Input and output in damped quantum systems: Quantum stochastic differential equations and the master equation. *Phys. Rev. A* **31**, 3761 (1985).
